# Supplementary material for: Modular session types for objects
Source: arXiv:1205.5344 source file (2015-12-23)
Supplement: Supplementary file 1 [file appendix.tex]

\appendix

\section*{Appendix: Proofs of lemmas from Section \ref{sec:techlemmas}}\label{app:proofs}

{
% numbering hacks

\renewcommand\label[1]{}

\inlineproofstrue
\explanatorytextfalse

\input{techlemmas}

} % end scope of redefinitions
